# Supplementary material for: Direct numerical simulation of pattern formation in subaqueous sediment
Source: arXiv:1405.5125 source file (2014-05-20)
Supplement: Supplementary file 1 [file additional_stuff.tex]

%%%%%%%%%%%%%%%%%%%%%%%%%%%%%%%%%%%%%%%%%%%%%%%%%%%%%%%%%%%%%%%%%%
%%%%%%%%%%%%%%%%55
\section{additional material}
%============================================================
% table: numerical parameters
%
\begin{table}
  \begin{center}
\def~{\hphantom{0}}
  \begin{tabular}{lcccccccc}
      Case &
      $[\Lx \times \Ly \times \Lz]/\Dia$  & 
      $N_x \times N_y \times N_z$  &   
      $\hmean/\Delta x$ &
      $\Delta x^+$ &
      $\Dia/\Delta x$ & 
      \Npm &
      \Npf &
      channel \\[3pt]
      \caseLa &
      $307.2\times 76.8\times 12.8$ & 
      $3072\times 769\times 128$ & 
      267.70 & 
      0.12 &
      10 &
      ~75531 &
      ~3542 &
      closed\\
      \caseLb &
      $307.2\times 76.8\times 12.8$ & 
      $3072\times 769\times 128$ & 
      265.33 &
      0.12 & 
      10 &
      ~75531 &
      ~3542 &
      closed\\
      \caseTa &
      $307.2\times 38.4\times 76.8$ & 
      $3072\times 385\times 768$ & 
      244.70 &
      1.07 & 
      10 &
      242160 &
      21252 &
      open\\
  \end{tabular}
  \caption{Numerical parameters of the sumulations.}
  \label{tab:numerical-parameters}
  \end{center}
\end{table}
%
% 
%============================================================
% figure: evolution of box kinetic energy
%
\begin{figure}
   \centering
       \begin{minipage}{2ex}
          \rotatebox{90}
          {\small $\langle k \rangle_{xyz}/\ubulk^2$}
        \end{minipage}
        \begin{minipage}{.43\linewidth}
          %\centerline{$(b)$}
          \includegraphics[width=\linewidth]
          {../plots/Box_averaged_kinetic_energy_ALL.pdf}
          \centerline{\small
            $t\cdot \ubulk/\hmean$}
        \end{minipage}%\\[20pt]
        \caption{
                 Time evolution of the box averaged 
                 turbulent kinetic 
                 energy.               
                 The simulation of case \caseTa\ was initially run
                 on a coarse grid while fixing the particles
                 in space (dashed-line in the plot).
                 The fully developed flow field was then refined to
                 the current grid resolution. 
                 Mobile particles
                 (except those at the bottom) were released first
                 at time $t=0$ thus insuring the flow field was
                 fully-developed (in the finer resolution)
                 when the particles were released ($t>0$).
                }
        \label{fig:time-evolution-of-kinetic-energy}
                                                                       
\end{figure}
%\clearpage
%
%============================================================
% figure: profiles of mean shear and velocity: L01 and T01
%
\begin{figure}
   \centering
        \raisebox{15ex}{$(a)$}
        \begin{minipage}{2ex}
          \rotatebox{90}
          {\small $(y-y_0)/\hmean$}
        \end{minipage}
        \begin{minipage}{.4\linewidth}
          %\centerline{$(a)$}
          \centerline{\mbox{}}
          \centerline{$\langle \tau \rangle /(\rho_f\ufric^2)$}
          \includegraphics[width=\linewidth]
          {../plots/Mean_Velocity_and_ShearProfile_laminar.pdf}
          \centerline{\small
            $\ufmean/\ubulk$}
        \end{minipage}
        \hspace{2ex}
        \raisebox{15ex}{$(b)$}
        \begin{minipage}{2ex}
          \rotatebox{90}
          {\small $(y-y_0)/\hmean$}
        \end{minipage}
        \begin{minipage}{.4\linewidth}
          %\centerline{$(b)$}
          \centerline{\mbox{}}
          \centerline{$\langle \tau \rangle /(\rho_f\ufric^2)$}
          \includegraphics[width=\linewidth]
          {../plots/Mean_Velocity_and_ShearProfile_turbulent.pdf}
          \centerline{\small
            $\ufmean/\ubulk$}
        \end{minipage}
        \caption{Wall-normal profiles of
                the mean streamwise fluid velocity (black) and
                total shear stress (blue).
                (\textit{a}), \caseLa; (\textit{b}) \caseTa.
                The total shear stress in case \caseTa is the sum
                of the viscous shear stress ({\color{blue}\dashed}) 
                and the Reynolds shear stress ({\color{blue}\chndot}). 
                The horizontal dashed lines show
                the offsets corresponding to the mean amplitude
                of the patterns ($\pm\hat{h}_{b,av}$). Friction
                velocity \ufric\ is determined by fitting a line
                to the linear region of $\langle \tau \rangle$ and
                extending it to $y_0$.
                }
        \label{fig:mean-velocity-and-shear-profile}
                                                                       
\end{figure}
%
%============================================================
% figure: evolution of particle flux
%
\begin{figure}
   \centering
       
         \raisebox{15ex}{$(b)$}
         \begin{minipage}{2ex}
          \rotatebox{90}
          {\small $\partflowrate/\flowrateref$}
        \end{minipage}
        \begin{minipage}{.43\linewidth}
          %\centerline{$(b)$}
          \includegraphics[width=\linewidth]
          {../plots/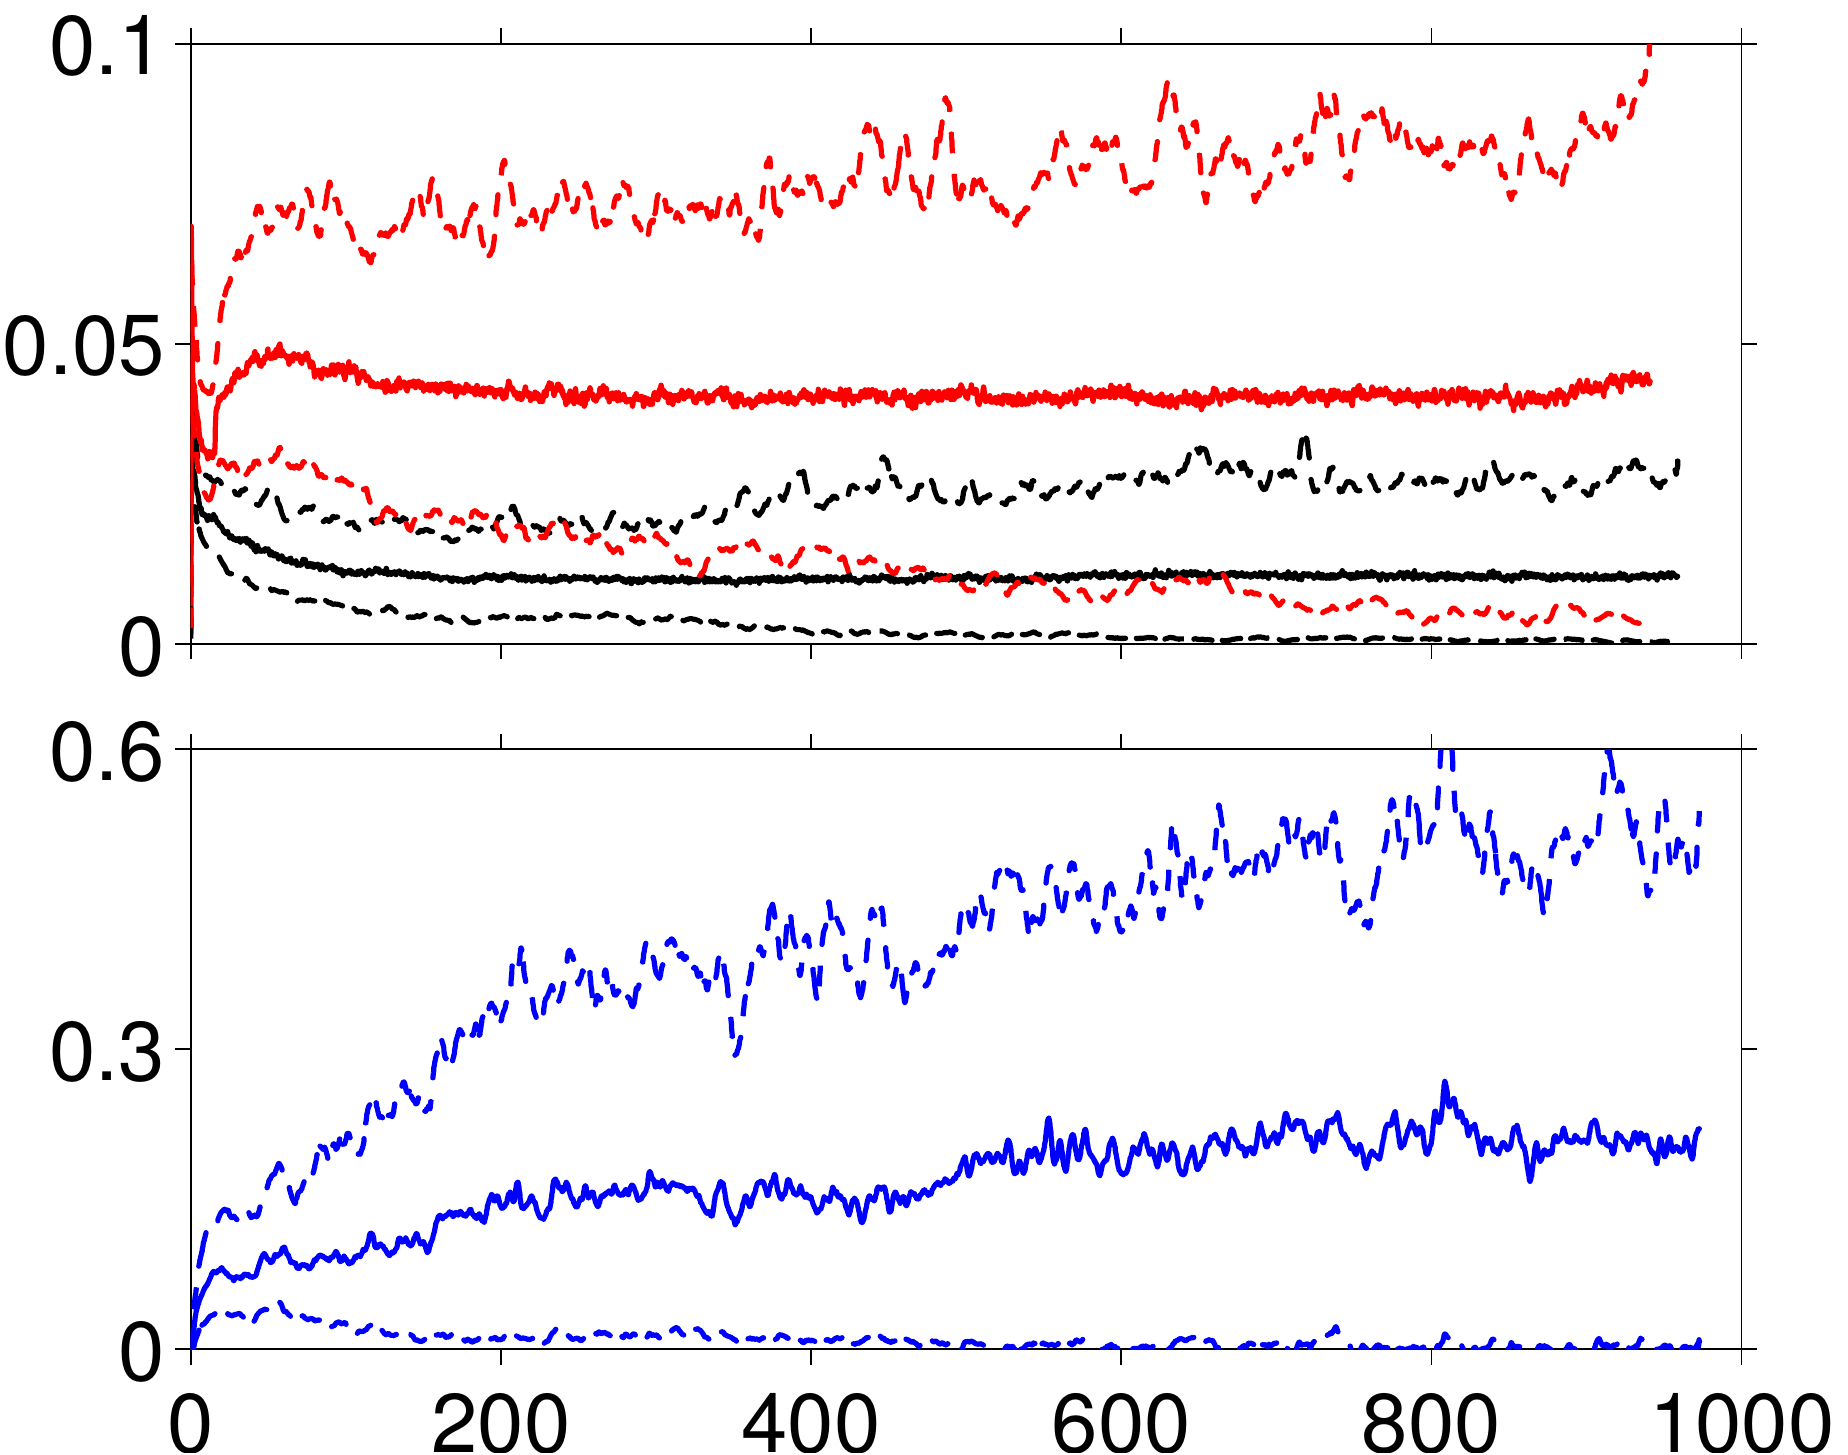}
          \centerline{\small
            $t\cdot \ubulk/\hmean$}
        \end{minipage}\\[20pt]
        \caption{
                 (\textit{b}) Time evolution of the particle
                  flux.
                }
        \label{fig:particle_flux_evolution}
                                                                       
\end{figure}
%
%============================================================
% figure: snapshot of the turbulent case z averaged slice
%
\begin{figure}
   \centering
        \begin{minipage}{2ex}
          \rotatebox{90}
          {\small $y/D$}
        \end{minipage}
        \begin{minipage}{.4\linewidth}
          %\centerline{$(a)$}
          \includegraphics[width=\linewidth]
          {../plots/slice_instant_ripple01Re3000_f0065_streamline.jpg}
          \centerline{\small
            $x/D$}
        \end{minipage}
         \begin{minipage}{2ex}
          \rotatebox{90}
          {\small $y/D$}
        \end{minipage}
         \begin{minipage}{0.4\linewidth}
          %\centerline{$(b)$}
          \includegraphics[width=\linewidth]
          {../plots/slice_zaveraged_ripple01Re3000_f0065_streamline.jpg}
          \centerline{\small
            $x/D$}
        \end{minipage}%\\[20pt]
        \caption{2D streamline plot in a closeup window for case T01.
                 (\textit{a}) for the data in figure
                 \ref{fig:instantaneous-snapshot-slice-instant-T01}.
                 (\textit{b}) for the data in figure
                 \ref{fig:instantaneous-snapshot-slice-zaveraged-T01}
                }
        \label{fig:streamline-plot-T01}
\end{figure}
%============================================================
% figure: snapshot of the turbulent case z averaged slice
%
\begin{figure}
   \centering
        \begin{minipage}{2ex}
          \rotatebox{90}
          {\small $y/D$}
        \end{minipage}
        \begin{minipage}{.7\linewidth}
          %\centerline{$(a)$}
          \includegraphics[width=\linewidth]
          {../plots/u_slice_instant_ripple01Re3000_f0065.jpg}
          %\centerline{\small
          %  $t\cdot u_b/h_f$;$\;t\cdot u_b/(2h_f)$}
        \end{minipage}\\[10pt]
         \begin{minipage}{2ex}
          \rotatebox{90}
          {\small $y/D$}
        \end{minipage}
         \begin{minipage}{0.7\linewidth}
          %\centerline{$(b)$}
          \includegraphics[width=\linewidth]
          {../plots/v_slice_instant_ripple01Re3000_f0065.jpg}
          \centerline{\small
            $x/D$}
        \end{minipage}%\\[20pt]
         \caption{(\textit{a})
                 Instantaneous snapshot of the
                 streamwise velocity in a plane located at 
                 $z=L_z/2$ for case T01. 
                 (\textit{b}) the same plot for wall-normal velocity}
        \label{fig:instantaneous-snapshot-slice-instant-T01}
\end{figure}
\begin{figure}
   \centering
        \raisebox{7ex}{$(d)$} 
        \begin{minipage}{2ex}
          \rotatebox{90}
          {\small $R_{\hbed^\prime\hbed^\prime}$}
        \end{minipage}
        \begin{minipage}{0.25\linewidth}
          %\centerline{(\textit{d})}
          \includegraphics[width=\linewidth]
          {../plots/Interface_correlation_selected_times_ripple01Re700.pdf}
          \centerline{\small $r_x/\Dia$ }
        \end{minipage}%\\[10pt]
        \hspace{1ex}
        \raisebox{7ex}{$(e)$} 
        \begin{minipage}{2ex}
          \rotatebox{90}
          {\small $R_{\hbed^\prime\hbed^\prime}$}
        \end{minipage}
        \begin{minipage}{0.25\linewidth}
         % \centerline{(\textit{e})}
          \includegraphics[width=\linewidth]
          {../plots/Interface_correlation_selected_times_ripple03Re700.pdf}
          \centerline{\small $r_x/\Dia$}
        \end{minipage}%\\[10pt]
        \hspace{1ex}
        \raisebox{7ex}{$(f)$} 
        \begin{minipage}{2ex}
          \rotatebox{90}
          {\small $R_{\hbed^\prime\hbed^\prime}$}
        \end{minipage}
        \begin{minipage}{0.25\linewidth}
         % \centerline{(\textit{f})}
          \includegraphics[width=\linewidth]
          {../plots/Interface_correlation_selected_times_ripple01Re3000.pdf}
          \centerline{\small $r_x/\Dia$}
        \end{minipage}\\
        \raisebox{12ex}{$(c)$} 
        \begin{minipage}{2ex}
          \rotatebox{90}
          {\small $\hat{h}_b/\Dia$}
        \end{minipage}
        \begin{minipage}{0.4\linewidth}
          %\centerline{(\textit{a})}
          \includegraphics[width=\linewidth]
        {../plots/Interface_dominant_amplitude_evolution_All.pdf}     
          \centerline{\small $t\cdot \ubulk/\hmean$ }
        \end{minipage}
        \hspace{1pt}
        \raisebox{12ex}{$(d)$} 
        \begin{minipage}{2ex}
          \rotatebox{90}
          {\small $d\varphi/dt\cdot(\lambda_x/2\pi)/\ubulk$}
        \end{minipage}
        \begin{minipage}{0.4\linewidth}
          %\centerline{(\textit{a})}
          \includegraphics[width=\linewidth]
        {../plots/Interface_dominant_phase_angle_evolution_All.pdf}     
          \centerline{\small $t\cdot \ubulk/\hmean$ }
        \end{minipage}
\end{figure}
%============================================================
% figure: slice snapshots of the turbulent case
%
\begin{figure}
   \centering
        \begin{minipage}{2ex}
          \rotatebox{90}
          {\small $y/D$}
        \end{minipage}
        \begin{minipage}{.7\linewidth}
          %\centerline{$(a)$}
          \includegraphics[width=\linewidth]
          {../plots/u_slice_zaveraged_ripple01Re3000_f0065.jpg}
          %\centerline{\small
          %  $t\cdot u_b/h_f$;$\;t\cdot u_b/(2h_f)$}
        \end{minipage}\\[10pt]
         \begin{minipage}{2ex}
          \rotatebox{90}
          {\small $y/D$}
        \end{minipage}
         \begin{minipage}{0.7\linewidth}
          %\centerline{$(b)$}
          \includegraphics[width=\linewidth]
          {../plots/v_slice_zaveraged_ripple01Re3000_f0065.jpg}
          \centerline{\small
            $x/D$}
        \end{minipage}%\\[20pt]
        \caption{(\textit{a})
                 Instantaneous snapshot of a spanwise-averaged
                 streamwise velocity for case T01. 
                 (\textit{b}) the same plot for wall-normal velocity}
        \label{fig:instantaneous-snapshot-slice-zaveraged-T01}
\end{figure}
